# Supplementary material for: Are Deep Neural Architectures Losing Information? Invertibility Is Indispensable
Source: arXiv:2009.03173 source file (2020-09-29)
Supplement: Supplementary file 1 [file supplementary.tex]

\begin{center}
{\LARGE\bfseries Supplementary Materials}

{\Large Are Deep Neural Architectures
Losing Information? \\
Invertibility Is Indispensable}
\end{center}

\section{Additional Figures}
